# Supplementary material for: Where to Focus: Query-Modulated Multimodal Keyframe Selection for Long Video Understanding
Source: arXiv:2604.17422 source file (2026-11-13)
Supplement: Supplementary file 1 [file appendix.tex]

%% 参考文献区域
\bibliographystyle{ACM-Reference-Format}
\bibliography{main}

%% --- 这里开始写附录 ---
\clearpage % 强制换页，让附录从新的一页开始
\appendix

\section{Extended Comparison of SOTA Methods}
\label{app:extended_comparison}

To provide a comprehensive overview of the current research landscape in long video keyframe selection, Table~\ref{tab:comparison_appendix} details the architectural and functional differences between Q-Gate and existing state-of-the-art paradigms. As discussed in the main text, while recent advancements have successfully introduced query-aware mechanisms, the vast majority of optimization-free frameworks remain fundamentally unimodal. They rely exclusively on visual features through either global semantic matching (e.g., AKS~\cite{tang2025adaptive}) or localized visual grounding (e.g., VSLS~\cite{guo2025logic}, T*~\cite{ye2025re}). Consequently, these baseline methods lack the structural capacity to process narrative context embedded within subtitles, rendering them ineffective for complex plot-driven reasoning tasks.

Beyond this unimodal limitation, existing selection mechanisms tend to be architecturally rigid. They typically employ static similarity thresholds or rely on computationally expensive agentic loops (e.g., Frame-Voyager~\cite{yu2024frame}) that require extensive policy training and incur unacceptable inference latency during practical deployment.

Q-Gate distinguishes itself as the first optimization-free framework to achieve a fully multimodal and query-modulated routing strategy. By concurrently integrating fine-grained visual grounding, global matching, and narrative context under an adaptive gated mechanism, Q-Gate effectively suppresses modality-specific noise. This dynamic coordination establishes a superior paradigm for scalable video reasoning and ensures precise evidence retrieval.

\begin{table*}[t]
\centering
\caption{Comprehensive comparison of state-of-the-art keyframe selection methods for long video understanding. \textbf{Q-Gate} is the first to introduce query-modulated gating that adaptively balances multi-granularity visual grounding and narrative context without requiring any training.}
\label{tab:comparison_appendix}
 
\resizebox{\textwidth}{!}{%  <--- 核心修复：强制等比例缩放至页面文字总宽度
\begin{tabular}{@{} lcccccc @{}} % <--- 核心修复：换回普通 tabular，去掉 fill
\toprule
\textbf{Method} & \textbf{Training-free} & \textbf{Query-aware} & \textbf{Multimodal} & \textbf{Fine-grained Grounding} & \textbf{Narrative Context} & \textbf{Selection Mechanism} \\
\midrule
Uniform          & \cmark & \xmark & \xmark & \xmark & \xmark & Static           \\
AKS~\cite{tang2025adaptive}   & \cmark & \cmark & \xmark & \xmark & \xmark & Similarity       \\
T*~\cite{ye2025re}         & \cmark & \cmark & \xmark & \cmark & \xmark & Iterative        \\
VSLS~\cite{guo2025logic}         & \cmark & \cmark & \xmark & \cmark & \xmark & Semantic        \\
Q-Frame~\cite{zhang2025q}   & \cmark & \cmark & \xmark & \xmark & \xmark & Resolution       \\
FOCUS~\cite{zhu2025focus}    & \cmark & \cmark & \xmark & \xmark & \xmark & MAB-Bandit       \\
\midrule
Frame-Voyager~\cite{yu2024frame} & \xmark & \cmark & \xmark & \xmark & \xmark & Agentic          \\
\midrule
\textbf{Q-Gate (Ours)} & \cmark & \cmark & \cmark & \cmark & \cmark & \textbf{Gated}   \\
\bottomrule
\end{tabular}%
}
\end{table*}

\section{Extended Implementation Details}
\label{app:implementation}

\subsection{Scoring Stream Architectures}
\label{app:stream_details}
To ensure full reproducibility and avoid task-specific training, our three scoring streams are implemented using publicly available, off-the-shelf vision and language models.

\begin{itemize}[leftmargin=1em, topsep=2pt, itemsep=0pt, parsep=0pt]
    \item \textbf{Visual Grounding ($S_g$)}: We employ the \textbf{YOLO-World}~\cite{cheng2024yolo} model with a ResNet-50 backbone. For each query, we first use a language model to extract key object nouns (e.g., ``cup'', ``woman''). The raw grounding score for each frame is calculated as the maximum detection confidence score among all target objects identified within that frame, prioritizing local, fine-grained visual details in frames.

    \item \textbf{Global Matching ($S_m$)}: To capture frame-level holistic semantics, we use the vision and text encoders from \textbf{BLIP-2}~\cite{li2023blip}, specifically the ViT-L/14 version. Each video frame and the textual query are encoded into their respective semantic spaces. The raw matching score is computed as the cosine similarity between these two embeddings.

    \item \textbf{Contextual Alignment ($S_c$)}: We leverage the \textbf{all-mpnet-base-v2} model from the Sentence-Transformers library~\cite{reimers2019sentence}, which is highly optimized for semantic textual similarity. The raw context score is computed as the cosine similarity between the query embedding and the embedding of the subtitle text that temporally aligns with the corresponding frame.
\end{itemize}

\subsection{Normalization and Fusion Parameters}
\label{app:norm_params}
The normalization pipeline is critical for mathematically aligning the heterogeneous raw scores from our three streams.
\begin{itemize}[leftmargin=1em, topsep=2pt, itemsep=0pt, parsep=0pt]
    \item \textbf{Min-Max Scaling}: A standard scaling maps all raw scores to a common range of $[0, 1]$.
    \item \textbf{Masked Temperature Softmax}: Across all experiments, we set the temperature $\mathbf{\tau = 0.5}$ to yield the optimal balance between noise suppression and frame diversity. The masking mechanism ensures that frames with an initial raw score of exactly zero (e.g., frames lacking subtitles for the Contextual stream) strictly remain at zero probability after the Softmax operation.
\end{itemize}

\section{Prompts for MLLM Inference}
\label{app:prompts}

\subsection{Query-Aware Gating Mechanism}
\label{app:gating_prompt}
The core of our dynamic fusion strategy relies on a sophisticated prompt that instructs an LLM (e.g., GPT-4o) to act as an expert router. The full prompt, detailed in Figure~\ref{fig:prompt_gating_appendix}, provides clear definitions of each expert stream's capabilities, explicitly dictates data-driven routing rules, and includes few-shot examples to ensure reliable JSON weight generation.

\begin{figure*}[h]
  \centering
  \includegraphics[width=0.95\textwidth]{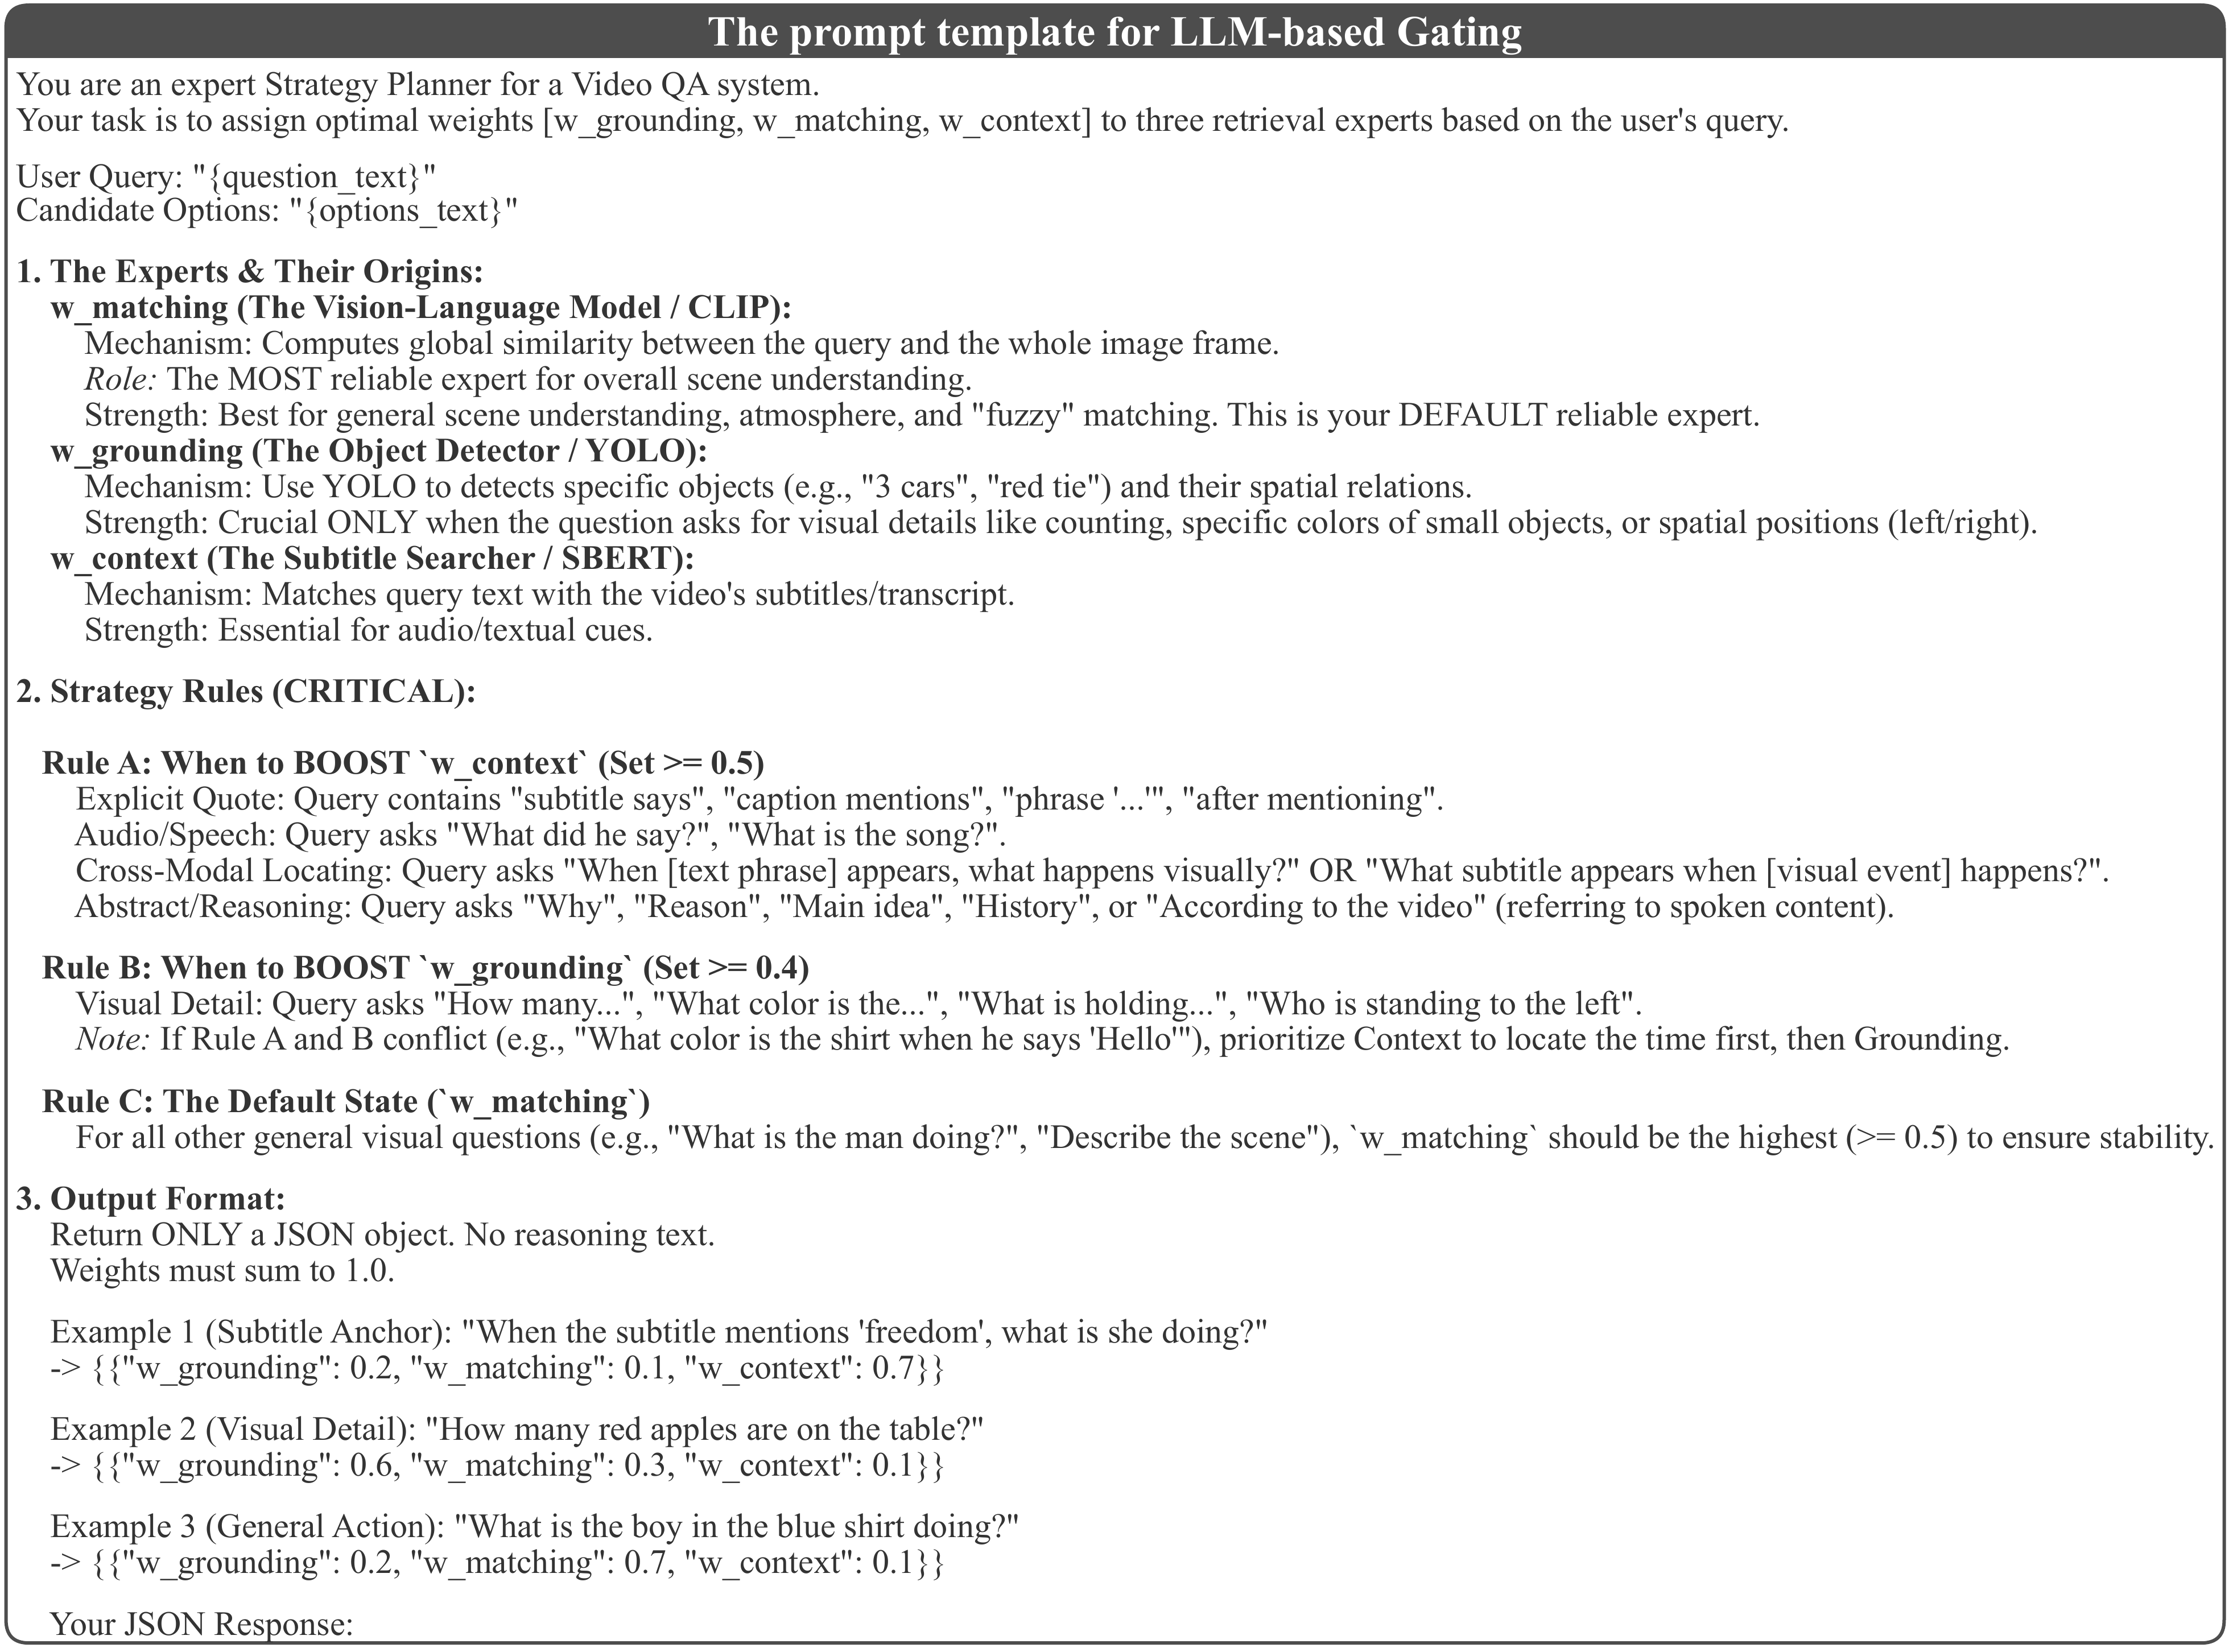} 
  \caption{The complete structured prompt template for our LLM-based Query-Aware Gating mechanism. By casting the LLM as an expert ``Strategy Planner,'' this prompt explicitly defines the functional boundaries and strengths of each retrieval expert. Furthermore, it incorporates empirically-derived strategy rules (Rules A-C) and diverse few-shot examples to rigorously guide the model's in-context reasoning. This carefully crafted design minimizes hallucination, ensures highly interpretable weight allocations based on user intent, and strictly enforces a machine-parsable JSON output.}
  \label{fig:prompt_gating_appendix}
\end{figure*}

\subsection{Downstream VLM Prompt}
\label{app:qa_prompt}
For the final question-answering stage, we employ a clean and direct prompt template (Figure~\ref{fig:prompt_qa_appendix}). A critical component of this prompt is the explicit inclusion of timestamps for both images (`[Image at MM:SS]') and subtitles (`[Subtitle for Image at MM:SS]'). This structure establishes a ``temporal bridge,'' enabling the downstream VLM to precisely align visual evidence with narrative context along the temporal axis.

\begin{figure*}[t] % 建议用 [t] 放在栏顶，最美观
  \centering
  \includegraphics[width=0.95\textwidth]{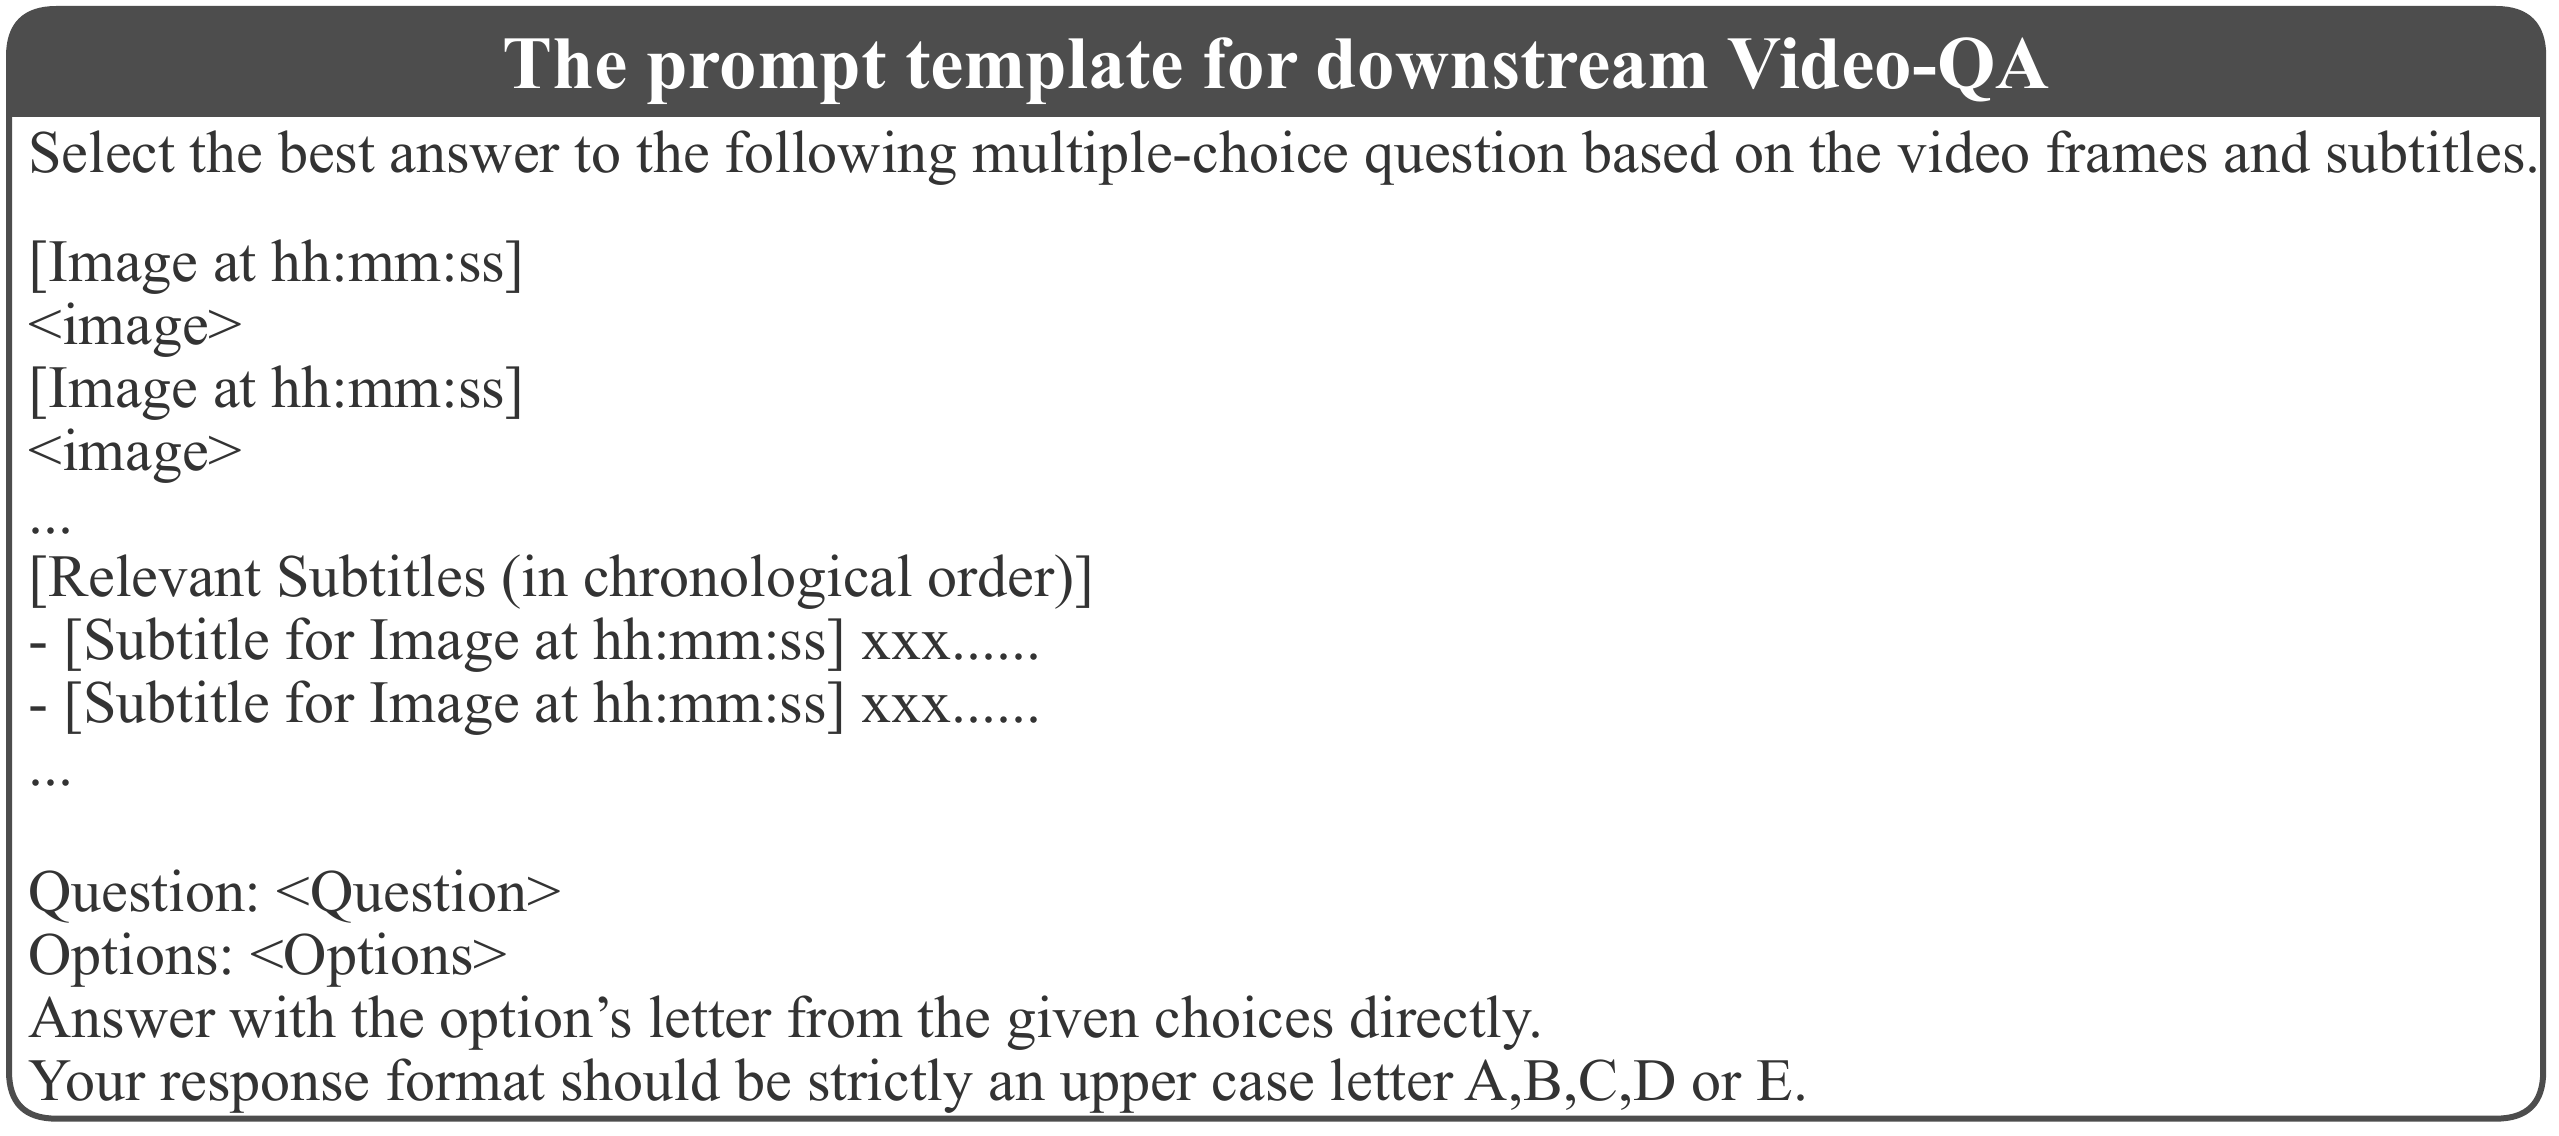} 
  \caption{The structured prompt template for downstream Video QA inference. By explicitly anchoring both visual frames and narrative subtitles with precise timestamps, this design constructs a crucial ``temporal bridge,'' empowering the VLM to perform seamless cross-modal reasoning and temporal verification.}
  \label{fig:prompt_qa_appendix}
\end{figure*}

\section{The Heuristic Gating Algorithm}
\label{app:heuristic}
While the LLM-based gating mechanism achieves the best performance, we also developed a lightweight Heuristic Gating Algorithm to provide a zero-latency alternative for latency-sensitive applications deployed in real-world scenarios.

\subsection{Algorithm Description}
The heuristic algorithm operates via rule-based keyword matching and score boosting:
\begin{sloppypar}
\begin{enumerate}[leftmargin=1.5em, topsep=2pt, itemsep=0pt, parsep=0pt]
    \item \textbf{Initialize Potentials}: It starts with a base potential score for each stream, with a default bias towards Global Matching (e.g., $p_{\mathrm{matching}}=1.0$).
    \item \textbf{Keyword-based Boosting}: It iterates through predefined sets of keywords. Queries containing ``how many'' or ``what color'' significantly boost $p_{\mathrm{grounding}}$, while queries with ``why'' or ``subtitle says'' boost $p_{\mathrm{context}}$.
    \item \textbf{Softmax Normalization}: The final potentials $[p_{\mathrm{grounding}}, p_{\mathrm{matching}}, p_{\mathrm{context}}]$ are passed through a Softmax function to produce the normalized weights $[w_g, w_m, w_c]$.
\end{enumerate}
\end{sloppypar}

\subsection{Performance Comparison}
\label{app:heuristic_performance}

As shown in Table~\ref{tab:gating_strategies_appendix}, the Heuristic Algorithm significantly outperforms the static ``Equal Weights'' baseline across all video lengths. This effectively demonstrates that even a straightforward, rule-based query analysis can successfully suppress modality-specific noise. While it slightly trails the powerful LLM Agent, its zero-latency nature makes it a highly practical and efficient choice for real-world deployments.

\begin{table}[h]
  \centering
  \caption{Comparison of Gating Strategies on LongVideoBench (GPT-4o, K=8). The Heuristic method provides a strong, efficient alternative to the LLM Agent, establishing a clear performance spectrum from static fusion to advanced dynamic LLM routing.}
  \label{tab:gating_strategies_appendix}
   % 稍微拉开行距，更美观
  \begin{tabular}{lccc}
    \toprule
    \textbf{Strategy} & \textbf{Long} & \textbf{Medium} & \textbf{Short} \\
    \midrule
    Static (Equal Weights) & 47.70 & 53.64 & 55.56 \\
    \textbf{Dynamic (Heuristic)} & 49.50 & 54.80 & 59.20 \\
    \textbf{Dynamic (LLM Agent)} & \textbf{50.71} & \textbf{56.55} & \textbf{65.41} \\
    \bottomrule
  \end{tabular}
\end{table}

\section{Limitations and Future Directions}
\label{app:limitations}

While Q-Gate demonstrates significant improvements in multi-modal video reasoning, our observations reveal several inherent challenges in the field that pave the way for future research:

\begin{itemize}[leftmargin=1em, topsep=2pt, itemsep=0pt, parsep=0pt]
    \item \textbf{Audio-Visual Temporal Misalignment}: In real-world videos, there is often a natural temporal lag between spoken dialogue and the corresponding visual action. While our Contextual stream precisely locates the subtitle cue, the selected frames might miss the visual climax due to this lag. Future work could explore temporally expanded sampling windows around textual anchors.
    
    \item \textbf{The Downstream Reasoning Bottleneck}: We observed instances where Q-Gate successfully extracts the ``ground-truth'' keyframes containing all necessary evidence, yet the downstream VLM still answers incorrectly. This indicates that overall video QA performance is increasingly bottlenecked by the inherent multi-hop reasoning capacity of current MLLMs.
    
    \item \textbf{Beyond Textual Audio Cues}: Our current ``Listen'' mechanism is limited to textual subtitles. It omits crucial non-speech audio cues (e.g., sound effects, background music) vital for understanding scene atmosphere. Integrating a dedicated audio event detection stream is a natural next step for a fully omni-modal routing framework.
    
    \item \textbf{Latency Distillation}: To eliminate the latency introduced by proprietary LLM gating, future research could distill the reasoning capabilities of this ``teacher'' model into a lightweight student network for instantaneous, on-device modality routing.
\end{itemize}

%% --- 附录结束 ---

\end{document}
